# Supplementary material for: Strong Formulations for Distributionally Robust Chance-Constrained Programs with Left-Hand Side Uncertainty under Wasserstein Ambiguity
Source: arXiv:2007.06750 source file (2021-01-13)
Supplement: Supplementary file 1 [file a.appendix.tex]

\section{Conic disjunctions}

By \eqref{eq:cc-distance-formulation}, the feasible region is
\begin{align*}
\cX_{\DR}(\cS) = \left\{ \vx \in \cX : \begin{aligned}
&\quad \exists\  t \geq 0, \ \vr \geq \bm{0},\\
&\quad \dist(\vxi^i,\cS(\vx)) \geq t - r^i, \ i \in [N],\\
&\quad \epsilon\, t \geq \theta + \frac{1}{N} \sum_{i \in [N]} r^i
\end{aligned} \right\}.
\end{align*}
By \eqref{eq:safety} and \eqref{eq:distance-linear}, the distance function is
\[ \dist(\vxi,\cS(\vx)) = \max\left\{ 0,\ \min_{p \in [P]} \frac{(\vb-\vA^\top \vx)^\top \vxi_p + d_p - \va_p^\top \vx}{\|\vb-\vA^\top \vx \|_*} \right\}. \]
This can be reformulated as
\[(\vx,\vr,t,u) \in \cX \times \bbR_+^N \times \bbR_+ \times \bbR_+ \quad \text{s.t.} \quad 
\begin{aligned}
&\epsilon t \geq \theta u + \frac{1}{N} \sum_{i \in [N]} r^i\\
&(\vx,r^i,t,u) \in S(\vxi^i)\\
&\|\vb - \vA^\top \vx\|_* \leq u
\end{aligned}
\]
where
\[ S(\vxi) = \left\{ (\vx,r,t,u) : \begin{aligned}
&(\vb - \vA^\top \vx)^\top \vxi_p + d_p - \va_p^\top \vx \geq t - r, \ \forall p \in [P]\\
&\|\vb - \vA^\top \vx\|_* \leq u
\end{aligned} \right\} \cup \left\{ (\vx,r,t,u) : \begin{aligned}
&0 \geq t - r\\
&\|\vb - \vA^\top \vx\|_* \leq u
\end{aligned} \right\}. \]

{\crd Nam: previously, I had explored disjunctions for the following set
\[ \left\{ (\vx,s,u) : \begin{aligned}
&\vx^\top \vxi - \alpha u \geq s\\
&\|\vx\|_* \leq u
\end{aligned} \right\} \cup \left\{ (\vx,s,u) : \begin{aligned}
&0 \geq s\\
&\|\vx\|_* \leq u
\end{aligned} \right\} \]
where $\alpha \geq 0$, and saw that it was related to an eigenvalue problem. I used conic disjunction results from Fatma's paper with Sam Burer.

The difference between this and $S(\vxi)$ is that $P=1$, $\vb - \vA^\top \vx = \vx$, $d_p - \va_p^\top x = 0$, and there is an additional $-\alpha u$ term in the linear part. I don't remember if $\alpha > 0$ was necessary for this, or whether it could work with $\alpha = 0$.
}
